# Supplementary material for: Staged Specification Logic for Verifying Higher-Order Imperative Programs (Technical Report)
Source: arXiv:2308.00988 source file (2024-07-02)
Supplement: Supplementary file 1 [file appendix-entm2.tex]

\newpage

\begin{verbatim}

Simplified Entailment Rules 
---------------------------
      D*D2|-(ex x*. D1*F)
      F |- (ex x*.S1) <: (ex y*.S2)
  -------------------------------------
    D |- ex x*. (req D1;S1)  <: ex y*. (req D2;S2) 

     D*D1|-(ex y*. D2*F)
      F |- (ex x*.S1) <: (ex y*.S2)
  -------------------------------------
    D |- ex x*. (ens D1;S1)  <: ex y*. (ens D2;S2) 

      emp&XP(D)&(v=w)* |- S1<:S2
  -----------------------------------------------
    D |- (ex x*. f$(v*);S1)  <: (ex y*. f$(w*);S2) 

Alternative way of proving soundness..
  Given forall c . {emp} c {F1} implies {emp} c {F2},
  we can conclude F1<:F2.

For 2-stages, it should be easy to show:
   D*D3|-D1*F        F*D2 |- D4*F2
 -------------------------------------
  emp |- req D1 ens D2 <: req D3 ens D4

For 2-stage pre/post logic, it is easy to show
        {D1} code {D2}
   ---------------------------
    {emp} code {req D1 ens D2} 

This is cause in Hoare logic, we can show.
   D1'|-D1*F  {D1} code {D2}  F*D2|-D2'
  ----------------------------------------
              {D1'} code {D2'}

Thus for 2-stage pre/post, we should be able to prove:
  Given forall c . {emp} c {req D1 ens D2} implies {emp} c {req D1' ens D2'},
  we can conclude emp |- req D1 ens D2 <: req D1' ens D2

Can we use above idea to prove more general case?

In general, we should also have the following structural rule:
    {S;ens D} code {S}
  --------------------
    {S} code {req D;S} 


    A * D |- D1 * R
    {A*R} code {S1}
 ----------------------
   {D} code {req D1;S1}

    x->a*y->b|-x->a * ?
    ? * x->1 |- ens x->1*y->b
 -----------------------------------------------------
 req x->a; ens x->1    <: req x->a*y->b; ens x->1*y->b

    x->a*a>2|-x->a * ?
    a>2 * x->a+1 |- x->b/\b>3
 -----------------------------------------------------
 req x->a; ens x->a+1    <: req x->a/\a>2; ens x->b/\ b>3
\end{verbatim}
