# Supplementary material for: Staged Specification Logic for Verifying Higher-Order Imperative Programs (Technical Report)
Source: arXiv:2308.00988 source file (2024-07-02)
Supplement: Supplementary file 2 [file appendixlabels.tex]

\newlabel{sec:elidedspecsexamples@cref}{{[subappendix][1][2147483647]A}{[1][16][]16}}
\newlabel{sec:casestudies@cref}{{[subappendix][3][2147483647]C}{[1][17][]17}}
\newlabel{sec:disjpre@cref}{{[subappendix][4][2147483647]D}{[1][18][]18}}
\newlabel{app:forward-ex@cref}{{[subappendix][5][2147483647]E}{[1][19][]19}}
\newlabel{app:cameleer-ex@cref}{{[subappendix][6][2147483647]F}{[1][20][]20}}
\newlabel{app:entail@cref}{{[subappendix][7][2147483647]G}{[1][21][]21}}
\newlabel{sec:inductive@cref}{{[subsubappendix][2][2147483647,7]G.2}{[1][23][]23}}
\newlabel{sec:lemmas@cref}{{[subappendix][8][2147483647]H}{[1][23][]23}}
\newlabel{sec:bigstep@cref}{{[subsubappendix][1][2147483647,9]I.1}{[1][24][]25}}
\newlabel{sec:norm_sound@cref}{{[subsubappendix][2][2147483647,9]I.2}{[1][25][]25}}
\newlabel{sec:forw_sound@cref}{{[subsubappendix][3][2147483647,9]I.3}{[1][25][]26}}
\newlabel{sec:entail_sound@cref}{{[subsubappendix][4][2147483647,9]I.4}{[1][27][]27}}
\newlabel{sec:term@cref}{{[subsubappendix][5][2147483647,9]I.5}{[1][28][]28}}
